# Supplementary material for: Hall mass and transverse Noether spin currents in noncollinear antiferromagnets
Source: arXiv:2404.12898 ancillary file (2024-12-25)
Supplement: Supplementary file 1 [file NoncollAFM_supp_rev1.pdf]

# Supplemental Material for "Hall mass and transverse Noether spin currents in noncollinear antiferromagnets"

Luke Wernert,[1] Bastian Pradenas,[2] Oleg Tchernyshyov,[2] and Hua Chen[1,3]

[1] *Department of Physics, Colorado State University, Fort Collins, CO 80523, USA*
[2] *William H. Miller III Department of Physics and Astronomy, Johns Hopkins University, Baltimore, MD 21218, USA*
[3] *School of Advanced Materials Discovery, Colorado State University, Fort Collins, CO 80523, USA*

## CONTENTS

I. Derivation of the Noether spin current formula using rotation matrices 1

II. On the spin current driving force $\mathcal{P}$ 2

III. Translation to the spin-frame notation 4

IV. Dynamical Noether Spin Current 5

V. Injection of magnons from FM to noncollinear AFM 8

VI. Derivation of the general formula of $\Gamma$ 11

VII. Spin waves and d.c. spin currents of isotropic noncollinear antiferromagnets 13

References 14

## I. DERIVATION OF THE NOETHER SPIN CURRENT FORMULA USING ROTATION MATRICES

In this section we derive the Noether spin current formula in the main text starting from the continuum Lagrangian, obtained by gradient-expanding the nearest-neighbor Heisenberg AFM model on the kagome lattice using the rotation matrix formalism. The gradient expansion has been done in several previous works [1–6] and will not be repeated here. The resulting Lagrangian given in the main text is invariant under global spin rotations acting on $R$. We can therefore use Noether's theorem to derive the conserved charge and currents due to the spin rotation or exchange symmetry. The general expression of the Noether current for a field theory of the multi-component field variable $\phi^i$ and the infinitesimal symmetry transformation parameterized by $\omega_a$ is [7]

$$\mathcal{J}^a_\mu = \left(\frac{\partial \mathcal{L}}{\partial(\partial_\mu \phi^i)}\partial_\nu\phi^i - \mathcal{L}\delta_{\mu\nu}\right)\frac{\partial x_\nu}{\partial \omega_a} - \frac{\partial \mathcal{L}}{\partial(\partial_\mu \phi^i)}F^i_a[\phi] \tag{1}$$

In the present case, $\omega_a$ corresponds to the infinitesimal rotation angle vector $\boldsymbol{\theta}$ defined through the transformation $R \to R' = (\mathbb{I} + \boldsymbol{\theta}\cdot\mathbf{L})R$, where the tensor $(L^\alpha)_{\beta\gamma} = -\epsilon_{\alpha\beta\gamma}$ is the generator of SO(3) rotations. Applying Eq. (1) to $\mathcal{L}$ for the spin rotation symmetry gives the Noether current density (a -1 factor is multiplied to the $\mathcal{J}^a_\mu$ for the correct sign of the conserved charge):

$$\mathcal{J}^\alpha_a = \frac{\partial \mathcal{L}}{\partial(\partial_a R_{\beta\gamma})}L^\alpha_{\beta\delta}R_{\delta\gamma} = \frac{1}{2}\mathrm{Tr}\left(\Gamma_{ab}R^{-1}L^\alpha\partial_b R\right) \tag{2}$$

where the trace is over spin indices that are left implicit. The corresponding conserved Noether charge density is

$$\mathcal{J}^\alpha_0 = \frac{\partial \mathcal{L}}{\partial(\partial_t R_{\beta\gamma})}L^\alpha_{\beta\delta}R_{\delta\gamma} = \rho\Omega_\alpha \tag{3}$$

By applying the Euler-Lagrange equation for the canting field [1, 2], we obtain

$$\mathcal{J}^\alpha_0 = \frac{1}{A_c}(S^\alpha_1 + S^\alpha_2 + S^\alpha_3) \tag{4}$$

The conserved charge density is therefore the net spin per unit cell area.

In practice the Noether spin current can be calculated for any given magnetic configurations represented by unit vectors $\hat{\mathbf{m}}_i$ along the spin directions on different sites, by writing $\Gamma$ in terms of the ground state spins $\mathbf{S}_{i0} = S\hat{\mathbf{m}}_{i0}$, and expressing $R\hat{\mathbf{m}}_{i0}$ as $\hat{\mathbf{m}}_i$. The spatial derivatives such as $\partial_j \mathbf{m}_{ia}$ can be approximated by finite difference [8]:

$$\partial_j \mathbf{m}_{ia} \approx \sum_{2\mathrm{nn}} \frac{a^j_{2\mathrm{nn}}}{3|\mathbf{a}_{2\mathrm{nn}}|^2}[\mathbf{m}_{(i+2\mathrm{nn})a} - \mathbf{m}_{ia}] \tag{5}$$

where 2nn stands for second nearest neighbor. The domain wall configuration illustrated in Fig. 1 below is obtained by adding easy-axis ($K$) and easy-plane ($K_z$) anisotropies to the spin Hamiltonian, [2]

$$H = J\sum_{\langle i,j\rangle} \mathbf{S}_i \cdot \mathbf{S}_j - K\sum_i (\hat{\mathbf{n}}_i \cdot \mathbf{S}_i)^2 + K_z \sum_i (\hat{\mathbf{z}} \cdot \mathbf{S}_i)^2 \tag{6}$$

fixing the spins on the left and right boundaries (periodic boundary condition is assumed for the top and bottom edges), followed by relaxing those in-between using Landau-Lifshitz-Gilbert equation.

Alternatively, for simple spatial dependence of $R$, such as

$$R(\mathbf{r}) = \begin{pmatrix} \cos(qx) & -\sin(qx) & 0 \\ \sin(qx) & \cos(qx) & 0 \\ 0 & 0 & 1 \end{pmatrix} \equiv R_z(qx) \tag{7}$$

where $q$ is a constant, one can directly use Eq. (2) and find that for the kagome models considered above the only nonzero component is

$$\mathcal{J}^z_x = -\frac{q}{2}\Gamma^{xx}_{xx} = -\frac{\sqrt{3}JS^2}{4}q \tag{8}$$

for both spin ordering. Similarly, for $R_x(qx)$ and $R_y(qx)$, we have

$$R_x(qx): \begin{cases} \mathcal{J}^y_y = \frac{q}{2}\Gamma^{yx}_{yx}\cos(qx) = \pm\frac{\sqrt{3}JS^2}{8}q\cos(qx) \\ \mathcal{J}^z_y = \frac{q}{2}\Gamma^{yx}_{yx}\sin(qx) = \pm\frac{\sqrt{3}JS^2}{8}q\sin(qx) \end{cases} \tag{9}$$

$$R_y(qx): \begin{cases} \mathcal{J}^y_x = -\frac{q}{2}\Gamma^{xx}_{xx} = -\frac{\sqrt{3}JS^2}{4}q \\ \mathcal{J}^x_y = \frac{q}{2}\Gamma^{xy}_{yx}\cos(qx) = \pm\frac{\sqrt{3}JS^2}{8}q\cos(qx) \\ \mathcal{J}^z_y = -\frac{q}{2}\Gamma^{xy}_{yx}\sin(qx) = \mp\frac{\sqrt{3}JS^2}{8}q\sin(qx) \end{cases}$$

where the upper and lower signs correspond to the direct and inverse triangular order, respectively.

Fig. 1 gives an example of the static spin currents near a domain wall, stabilized by an additional anisotropy term in the energy functional [2] and calculated using finite difference, Eq. (5). One can find that $\mathcal{J}^x_z$ is predominantly large compared to the other components as expected from the analytic results above. The other nonzero components are partly due to $H_{\mathrm{ani}}$ that acts as source/sink of $\mathcal{J}$ and partly to the finite difference approximation employed.

## II. ON THE SPIN CURRENT DRIVING FORCE $\mathcal{P}$

In this section we discuss in more detail the meaning of the driving force $\mathcal{P}$

$$(\mathcal{P}^\alpha_b)_{\beta\gamma} = \frac{1}{2}(R^{-1}L^\alpha \partial_b R)_{\beta\gamma} \tag{10}$$

We assume the reader is familiar with the essential terminology of gauge theory [7]. Gauge potential or connection originates from the discussion of parallel transport. Suppose we have a field theory for $\phi(x)$ which defines a mapping from a base manifold $M$ to a target manifold $F$, and has a gauge group $G$. An infinitesimal parallel transporter $\Lambda \in G$ can be written as

$$\Lambda = \mathbb{I} - \epsilon A \tag{11}$$

where $\epsilon$ is an infinitesimal number, and $A$ is an element of the Lie algebra of $G$. The requirement of gauge invariance under an arbitrary $g \in G$, which acts on $\phi$ from its left, requires $A$ to transform as:

$$A \to A' = gAg^{-1} + gdg^{-1} \tag{12}$$

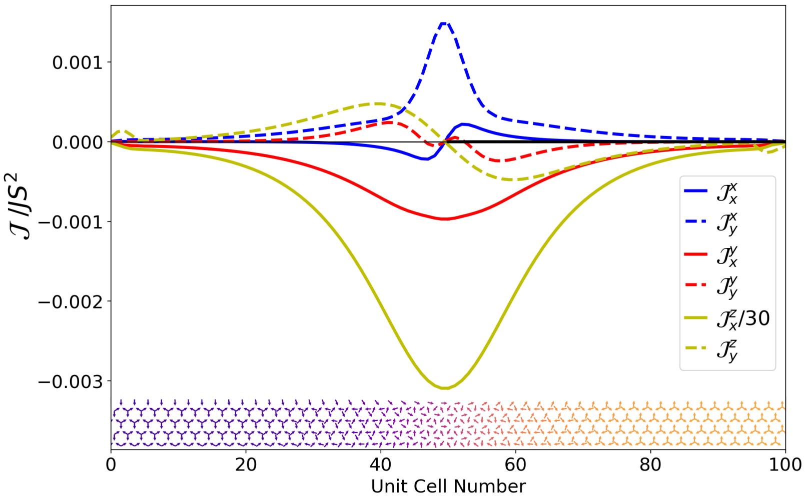


FIG. 1. Static Noether spin current near a domain wall in the 2D kagome model with the direct triangular AFM order illustrated in the inset. $\mathcal{J}_x^z$ is predominantly large and is rescaled by a factor of $1/30$ for better visualization.

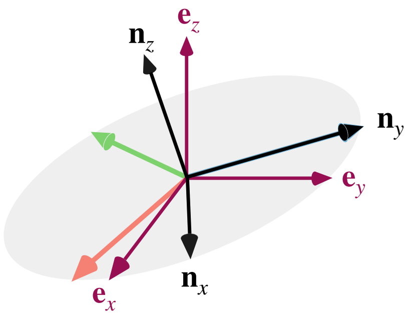


FIG. 2. Global and Body-axes. The shaded arrows in RGB illustrate the magnetization vectors of the sublattice. Vectors depicted in a darker shade correspond to the spin frame vectors (local frame), analogous to the principal axis of a rigid body. The vectors colored in purple represent the fixed Cartesian axes (global frame). The matrices of angular momentum, $L^\alpha$ generate rotations around the global axes Eq. (17), whereas the matrices $R^{-1}L^\alpha R$ induce rotations around the body axes Eq. (19).

in the notation of differential forms.

We next consider the connection of SO(3) due to rotating the internal or local frame (Fig. 2), which amounts to

$$R \to R' = Rg \tag{13}$$

Therefore for infinitesimal $\Lambda$, which is also a local frame rotation, we have

$$A' = g^{-1}Ag - g^{-1}dg \tag{14}$$

For the gauge potential due to spin waves considered here, we can take $A = 0$. As a result, the gauge potential can be chosen as

$$A = -R^{-1}dR \tag{15}$$

or $A_b = -R^{-1}\partial_b R$ where $R = R[\boldsymbol{\theta}(\mathbf{r}, t)] \approx \mathbb{I} + \boldsymbol{\theta}\cdot\mathbf{L} + \frac{1}{2}(\boldsymbol{\theta}\cdot\mathbf{L})^2$ is the infinitesimal rotation due to the spin waves. $A_b$ is a rank-3 tensor. But since $A_b = -A_b^T$, we can just keep its 3 antisymmetric components and convert it to a vector (for a given $b$) [9]:

$$a_b^\alpha \equiv -\frac{1}{2}\epsilon_{\alpha\beta\gamma}(R^{-1}\partial_b R)_{\beta\gamma} = -\frac{1}{2}\mathrm{Tr}(L^\alpha R^{-1}\partial_b R). \tag{16}$$

More generally, since $A_b$ is an element of so(3) Lie algebra, it can be written as a vector in the basis of $L^\alpha$

$$A_b = -a_b^\alpha L^\alpha \tag{17}$$

Using $\mathrm{Tr}(L^\alpha L^\beta) = -2\delta_{\alpha\beta}$, we have

$$\frac{1}{2}\mathrm{Tr}(L^\alpha A_b) = a_b^\alpha \tag{18}$$

consistent with Eq. (16).

To see how $\mathcal{P}$ can be connected with the discussion above, we consider the Lie algebra spanned by $R^{-1}L^\alpha R$, which also satisfies the commutation relation $[(R^{-1}L^\alpha R),(R^{-1}L^\beta R)] = \epsilon_{\alpha\beta\gamma}(R^{-1}L^\gamma R)$ and $\mathrm{Tr}[(R^{-1}L^\alpha R)(R^{-1}L^\beta R)] = -2\delta_{\alpha\beta}$. As a result

$$\begin{aligned} A_b &= \frac{1}{2}\mathrm{Tr}[(R^{-1}L^\alpha R)(-R^{-1}\partial_b R)](-R^{-1}L^\alpha R) \\ &\equiv \tilde{a}_b^\alpha \tilde{L}^\alpha \end{aligned} \tag{19}$$

To see what $\tilde{L}^\alpha$ means, we consider the rotation generated by exponentiating it

$$e^{\boldsymbol{\phi}\cdot\tilde{\mathbf{L}}} = \exp\left[-\phi_\alpha(R^{-1}L^\alpha R)\right] = \exp\left[(-R^{-1}\boldsymbol{\phi})\cdot\mathbf{L}\right] \tag{20}$$

where we have used $R^{-1}L^\alpha R = R_{\alpha\beta}L^\beta$. Therefore $\tilde{\mathbf{L}}$ generates rotations by $-R^{-1}\boldsymbol{\phi}$. Since $\boldsymbol{\phi}$ is a Cartesian vector defined in the global frame, and $R$ describes the instantaneous orientation of the rigid body in the global frame, $R^{-1}\boldsymbol{\phi}$ describes the rotation angle vector in the instantaneous local frame, and the minus sign in $-R^{-1}\boldsymbol{\phi}$ means the resulting rotation is a right (or counter) rotation. Taken together, one can see that $\tilde{\mathbf{L}}$ generates local-frame rotations. We can therefore conclude that $\tilde{a}_b^\alpha$ is the coordinates of $A_b$, an SO(3) gauge potential due to spin waves understood as local-frame rotations, in the so(3) Lie algebra spanned by the local-frame rotation generators $\tilde{\mathbf{L}} = -(R^{-1}\mathbf{L}R)$. Since

$$a_b^\alpha = -\frac{1}{2}\mathrm{Tr}[(R^{-1}L^\alpha R)(R^{-1}\partial_b R)] = -\mathrm{Tr}(\mathcal{P}_b^\alpha) \tag{21}$$

$\mathcal{P}_b^\alpha$ can be understood as a projection (up to a minus sign) of the SO(3) gauge potential $A_b$ to the local-frame-rotation so(3) basis vector $\tilde{L}^\alpha$.

It is also illustrative to arrive at the above conclusion using global rotations. When we understand the spin wave rotation matrix $R$ as global rotations, the gauge potential due to spatial translation will be, according to Eq. (12):

$$A_b = R\partial_b R^{-1} = -(\partial_b R)R^{-1} \tag{22}$$

which is an element of the so(3) Lie algebra spanned by the regular global frame rotations $\mathbf{L}$:

$$A_b = a_b^\alpha L^\alpha = \frac{1}{2}\mathrm{Tr}[L^\alpha(\partial_b R)R^{-1}]L^\alpha \tag{23}$$

Therefore

$$a_b^\alpha = \mathrm{Tr}(R\mathcal{P}_b^\alpha R^{-1}) \tag{24}$$

Namely, $\mathcal{P}_b^\alpha$ can be understood as the projection of $A_b$ onto $L^\alpha$ written in the spin-wave local frame coordinates:

$$\mathcal{P}_b^\alpha = R^{-1}\left[\frac{1}{2}L^\alpha(\partial_b R)R^{-1}\right]R \tag{25}$$

## III. TRANSLATION TO THE SPIN-FRAME NOTATION

In this section, we translate the expressions of the SO(3) matrix field theory [1] to the language of spin frames [6]. A spin frame is a right triple of mutually orthogonal unit vectors $\mathbf{n}_\mu$ with labels $\mu = x, y, z$ and components $n_{\mu m}$, where $m = x, y, z$ labels spatial directions. The dichotomy of Latin indices for orbital (lattice) directions and Greek indices for spin directions is used to stress the lack of spin-orbit coupling in the exchange-only model.

An SO(3) rotation matrix $R$ takes the original unit vectors to their new orientations:

$$\mathbf{n}_x = \begin{pmatrix}1\\0\\0\end{pmatrix} \mapsto \begin{pmatrix}n_{x1}\\n_{x2}\\n_{x3}\end{pmatrix}, \quad \mathbf{n}_y = \begin{pmatrix}0\\1\\0\end{pmatrix} \mapsto \begin{pmatrix}n_{y1}\\n_{y2}\\n_{y3}\end{pmatrix}, \quad \mathbf{n}_z = \begin{pmatrix}0\\0\\1\end{pmatrix} \mapsto \begin{pmatrix}n_{z1}\\n_{z2}\\n_{z3}\end{pmatrix}. \tag{26}$$

Thus

$$R = \begin{pmatrix} n_{x1} & n_{y1} & n_{z1} \\ n_{x2} & n_{y2} & n_{z2} \\ n_{x3} & n_{y3} & n_{z3} \end{pmatrix}. \tag{27}$$

Component-wise, $n_{\mu m} = R_{m\mu} = (R^{-1})_{\mu m}$.

We thus obtain

$$\begin{aligned}(R^{-1}\partial_a R\, R^{-1}\partial_b R)_{\mu\nu} &= (R^{-1})_{\mu m}(\partial_a R)_{m\rho}(R^{-1})_{\rho n}(\partial_b R)_{n\nu} = n_{\mu m}\,\partial_a n_{\rho m}\, n_{\rho n}\,\partial_b n_{\nu n} \\ &= (\mathbf{n}_\mu\cdot\partial_a\mathbf{n}_\rho)(\mathbf{n}_\rho\cdot\partial_b\mathbf{n}_\nu) = -(\partial_a\mathbf{n}_\mu\cdot\mathbf{n}_\rho)(\mathbf{n}_\rho\cdot\partial_b\mathbf{n}_\nu) = -\partial_a\mathbf{n}_\mu\cdot\partial_b\mathbf{n}_\nu.\end{aligned} \tag{28}$$

Here we used the identity $\partial_a(\mathbf{n}_\mu\cdot\mathbf{n}_\rho) = 0$ for orthonormal vectors $\mathbf{n}_\mu\cdot\mathbf{n}_\rho = \delta_{\mu\rho}$ and the completeness of the spin-frame basis.

This result establishes the translation between the expressions for exchange energy density in the two languages:

$$\mathcal{U} = -\frac{1}{4}\Gamma^{\alpha\beta}_{ab}(R^{-1}\partial_a R\, R^{-1}\partial_b R)_{\alpha\beta} = \frac{1}{4}\Gamma^{\alpha\beta}_{ab}\partial_a\mathbf{n}_\alpha\cdot\partial_b\mathbf{n}_\beta. \tag{29}$$

## IV. DYNAMICAL NOETHER SPIN CURRENT

In this section we consider the Noether spin current due to dynamical spins and dicuss how to calculate it numerically for a lattice model. We start by deriving the relation between spin current and energy-momentum tensor using the spin-frame language. The Lagrangian density is

$$\mathcal{L} = \frac{\rho}{4}\,\partial_t\mathbf{n}_\alpha\cdot\partial_t\mathbf{n}_\alpha - \frac{1}{4}\Gamma^{\alpha\beta}_{ab}\,\partial_a\mathbf{n}_\alpha\cdot\partial_b\mathbf{n}_\beta \tag{30}$$

Here $\alpha,\beta,\ldots = x,y,z$ label spin-frame vectors, while $a,b,\ldots = x,y$ label spatial dimensions.

From Noether's theorem, we obtain the conserved spin current

$$\boldsymbol{\mathcal{J}}_i = \mathbf{n}_\alpha\times\frac{\partial\mathcal{L}}{\partial(\partial_i\mathbf{n}_\alpha)}. \tag{31}$$

Its temporal and spatial components are

$$\boldsymbol{\mathcal{J}}_0 = \frac{\rho}{2}\,\mathbf{n}_\alpha\times\partial_t\mathbf{n}_\alpha, \quad \boldsymbol{\mathcal{J}}_a = -\frac{1}{2}\Gamma^{\alpha\beta}_{ab}\,\mathbf{n}_\alpha\times\partial_b\mathbf{n}_\beta. \tag{32}$$

The energy-momentum tensor gives the density of linear momentum and energy,

$$\mathcal{T}_{a0} = -\frac{\rho}{2}\,\partial_t\mathbf{n}_\alpha\cdot\partial_a\mathbf{n}_\alpha, \quad \mathcal{T}_{00} = \frac{\rho}{4}\,\partial_t\mathbf{n}_\alpha\cdot\partial_t\mathbf{n}_\alpha + \frac{1}{4}\Gamma^{\alpha\beta}_{ab}\,\partial_a\mathbf{n}_\alpha\cdot\partial_b\mathbf{n}_\beta. \tag{33}$$

Consider a spin wave with frequency $\omega$, wavevector $\mathbf{k} = (k_x, k_y)$, and an elliptical polarization specified by two mutually orthogonal angular amplitudes $\boldsymbol{\theta}_1$ and $\boldsymbol{\theta}_2$:

$$\begin{aligned}\delta\mathbf{n}_\alpha &= [\boldsymbol{\theta}_1\cos(\omega t - k_a x^a) + \boldsymbol{\theta}_2\sin(\omega t - k_a x^a)]\times\mathbf{n}_\alpha, \\ \partial_t\delta\mathbf{n}_\alpha &= \omega[\boldsymbol{\theta}_2\cos(\omega t - k_a x^a) - \boldsymbol{\theta}_1\sin(\omega t - k_a x^a)]\times\mathbf{n}_\alpha, \\ \partial_\alpha\delta\mathbf{n}_\alpha &= -k_a[\boldsymbol{\theta}_2\cos(\omega t - k_a x^a) - \boldsymbol{\theta}_1\sin(\omega t - k_a x^a)]\times\mathbf{n}_\alpha.\end{aligned} \tag{34}$$

The spin density, averaged over a period of oscillation, is

$$\langle\boldsymbol{\mathcal{J}}_0\rangle = \frac{\rho}{2}\,\langle(\mathbf{n}_\alpha + \delta\mathbf{n}_\alpha)\times\partial_t\delta\mathbf{n}_\alpha\rangle = \frac{\rho\omega}{2}(\boldsymbol{\theta}_1\times\mathbf{n}_\alpha)\times(\boldsymbol{\theta}_2\times\mathbf{n}_\alpha) = \frac{\rho\omega}{2}\,\boldsymbol{\theta}_1\times\boldsymbol{\theta}_2. \tag{35}$$

The spatial components of the spin current are

$$\langle\boldsymbol{\mathcal{J}}_a\rangle = \frac{1}{2}\Gamma^{\alpha\beta}_{ab}\,k_b\,(\boldsymbol{\theta}_1\times\mathbf{n}_\alpha)\times(\boldsymbol{\theta}_2\times\mathbf{n}_\beta) = \frac{1}{2}\Gamma^{\alpha\beta}_{ab}\,k_b\,P_{\alpha\beta}\,(\boldsymbol{\theta}_1\times\boldsymbol{\theta}_2). \tag{36}$$

Here

$$P_{\alpha\beta}\boldsymbol{\theta} = \frac{1}{2}\mathbf{n}_\alpha(\mathbf{n}_\beta\cdot\boldsymbol{\theta}) + \frac{1}{2}\mathbf{n}_\beta(\mathbf{n}_\alpha\cdot\boldsymbol{\theta}). \tag{37}$$

We also assumed that $\Gamma^{\alpha\beta}_{ab} = \Gamma^{\beta\alpha}_{ab}$.

The densities of linear momentum and energy are

$$\langle\mathcal{T}_{a0}\rangle = \frac{1}{2}\rho\omega k_a\,(\boldsymbol{\theta}_1\cdot\boldsymbol{\theta}_1 + \boldsymbol{\theta}_2\cdot\boldsymbol{\theta}_2), \quad \langle\mathcal{T}_{00}\rangle = \frac{1}{2}\rho\omega^2(\boldsymbol{\theta}_1\cdot\boldsymbol{\theta}_1 + \boldsymbol{\theta}_2\cdot\boldsymbol{\theta}_2). \tag{38}$$

We used the equipartition theorem in the derivation of the latter.

The spin current and energy-momentum tensor of the spin wave satisfy the identity

$$\rho\,\langle\mathcal{T}_{00}\rangle\langle\boldsymbol{\mathcal{J}}_a\rangle = \Gamma^{\alpha\beta}_{ab}\,\langle\mathcal{T}_{b0}\rangle P_{\alpha\beta}\langle\boldsymbol{\mathcal{J}}_0\rangle. \tag{39}$$

The above derivation can be done similarly using the rotation matrix approach as we show below, where we also discuss the subtlety of keeping quadratic terms in $\boldsymbol{\theta}$ in the derivation. We make use of the exponential map $R(\boldsymbol{\theta}) = \exp(\boldsymbol{\theta}\cdot\mathbf{L})$ and obtain the second order in $\theta$ terms by expanding it

$$R(\boldsymbol{\theta}) \approx \mathbb{I} + \boldsymbol{\theta}\cdot\mathbf{L} + \frac{1}{2}(\boldsymbol{\theta}\cdot\mathbf{L})^2 \tag{40}$$

which is still an orthogonal matrix up to $O(\theta^2)$:

$$\begin{aligned} RR^T &= \left[\mathbb{I} + \boldsymbol{\theta}\cdot\mathbf{L} + \frac{1}{2}(\boldsymbol{\theta}\cdot\mathbf{L})^2\right]\left[\mathbb{I} - \boldsymbol{\theta}\cdot\mathbf{L} + \frac{1}{2}(\boldsymbol{\theta}\cdot\mathbf{L})^2\right] \\ &= \mathbb{I} + O(\theta^3) = R^T R \end{aligned} \tag{41}$$

Using the second order formula of $R$, we have

$$\begin{aligned} \partial_t R_{\alpha\beta} &= -\dot\theta_\gamma\epsilon_{\gamma\alpha\beta} + \frac{1}{2}(\dot\theta_\alpha\theta_\beta + \theta_\alpha\dot\theta_\beta - 2\theta_\gamma\dot\theta_\gamma\delta_{\alpha\beta}) \\ \Omega_\alpha &= \dot\theta_\alpha + \frac{1}{2}\epsilon_{\alpha\beta\gamma}\theta_\beta\dot\theta_\gamma + O(\theta^3) \\ (R^{-1}\partial_a R)_{\alpha\beta} &= -\epsilon_{\gamma\alpha\beta}\partial_a\theta_\gamma + \frac{1}{2}(\theta_\alpha\partial_a\theta_\beta - \theta_\beta\partial_a\theta_\alpha) + O(\theta^3) \\ (R^{-1}L^\gamma\partial_a R)_{\alpha\beta} &= \partial_a\theta_\alpha\delta_{\gamma\beta} - \partial_a\theta_\gamma\delta_{\alpha\beta} - \theta_\gamma\partial_a\theta_e\epsilon_{e\alpha\beta} - (\boldsymbol{\theta}\times\partial_a\boldsymbol{\theta})_\beta\delta_{\alpha\gamma} - \frac{1}{2}\partial_a(\theta_c\theta_\beta\epsilon_{\gamma\alpha c} - \theta^2\epsilon_{\gamma\alpha\beta}) + O(\theta^3) \end{aligned} \tag{42}$$

We next use Eq. (42) to derive the time average of various conserved quantities for spin waves $\boldsymbol{\theta}(\mathbf{r},t) = \mathrm{Re}[\boldsymbol{\theta}e^{i(\mathbf{k}\cdot\mathbf{r}-\omega t)}]$.

First consider the spin currents. The temporal component is

$$\begin{aligned} \langle\mathcal{J}^\alpha_0\rangle &= \rho\langle\Omega_\alpha\rangle = \frac{\rho}{2}\langle(\boldsymbol{\theta}\times\dot{\boldsymbol{\theta}})_\alpha\rangle \\ &= -\frac{\rho\omega}{4}\mathrm{Im}(\boldsymbol{\theta}\times\boldsymbol{\theta}^*)_\alpha \end{aligned} \tag{43}$$

The spatial components are

$$\begin{aligned} \langle\mathcal{J}^\alpha_a\rangle &= \frac{1}{2}\Gamma^{\beta\gamma}_{ab}\langle(R^{-1}L^\alpha\partial_b R)_{\beta\gamma}\rangle \\ &= \frac{1}{2}\Gamma^{\beta\gamma}_{ab}\langle-(\boldsymbol{\theta}\times\partial_b\boldsymbol{\theta})_\gamma\delta_{\alpha\beta} - \frac{1}{2}\partial_b(\theta_\lambda\theta_\gamma)\epsilon_{\alpha\beta\lambda}\rangle \\ &= -\frac{1}{4}\Gamma^{\alpha\beta}_{ab}\mathrm{Im}(\boldsymbol{\theta}\times\boldsymbol{\theta}^*)_\beta \end{aligned} \tag{44}$$

where we have used the symmetry of $\Gamma^{\alpha\beta}_{ab} = \Gamma^{\beta\alpha}_{ab}$. Note that keeping only the $O(\theta^1)$ term in the expansion of $R$ leads to the same results.

$\langle\mathcal{T}_{00}\rangle$ and $\langle\mathcal{T}_{b0}\rangle$ can be calculated similarly. The equivalence between the two approaches can be seen explicitly by using $\mathbf{n}_{x,y,z} = \hat{\mathbf{x}}, \hat{\mathbf{y}}, \hat{\mathbf{z}}$.

To calculate the dynamical spin current using Eq. (44) for a lattice model, we start from the LLG equation

$$\dot{\mathbf{m}} = -\gamma \mathbf{m} \times \mathbf{H}_{\text{eff}} + \frac{\alpha}{|\mathbf{m}|}\mathbf{m} \times \dot{\mathbf{m}} \tag{45}$$

where the effective field $\mathbf{H}_{\text{eff}}$ depends on both the field-free Hamiltonian $H(\{\mathbf{m}_i\})$ and any position-dependent external magnetic fields $\mathbf{h}_i^{\text{ext}}$, taken as a perturbation. We then linearize the LLG equation by keeping only first order in $\delta\mathbf{m}_i \equiv \mathbf{m}_i - \mathbf{m}_i^0$ and $\mathbf{h}_i^{\text{ext}}$ terms:

$$\frac{d}{dt}\delta\mathbf{m}_i = \gamma\delta\mathbf{m}_i \times \frac{\partial H}{\partial \mathbf{m}_i^0} + \gamma\mathbf{m}_i^0 \times \sum_j \frac{\partial^2 H}{\partial\mathbf{m}_i^0 \partial\mathbf{m}_j^0} \cdot \delta\mathbf{m}_j - \gamma\mathbf{m}_i^0 \times \mathbf{h}_i^{\text{ext}}(t) + \frac{\alpha}{|\mathbf{m}_i^0|}\mathbf{m}_i^0 \times \frac{d}{dt}\delta\mathbf{m}_i \tag{46}$$

Setting $\delta\mathbf{m}_i(t) = \delta\mathbf{m}_i e^{-i\omega t}$, $\mathbf{h}_i^{\text{ext}}(t) = \mathbf{h}_i^{\text{ext}} e^{-i\omega t}$ and grouping together like terms provides

$$\sum_j \left[-i\omega\delta_{ij} + \gamma\delta_{ij}\left(\frac{\partial H}{\partial\mathbf{m}_i^0}\times\right) - \gamma\left(\mathbf{m}_i^0 \times \frac{\partial^2 H}{\partial\mathbf{m}_i^0\partial\mathbf{m}_j^0}\cdot\right) + i\omega\delta_{ij}\frac{\alpha}{|\mathbf{m}_i^0|}\left(\mathbf{m}_i^0\times\right)\right]\delta\mathbf{m}_j = -\gamma\mathbf{m}_i^0 \times \mathbf{h}_i^{\text{ext}} \tag{47}$$

Although Eq. (47) can be directly inverted due to the presence of $\alpha$, it is better to eliminate the redundant longitudinal degrees of freedom first. To this end we arbitrarily pick a set of unit vectors $\{\hat{n}_i\}$ in a way that $\hat{n}_i \times \mathbf{m}_i^0 \neq 0$. When $\mathbf{m}_i^0$ are collinear or coplanar a single $\hat{n}$ is sufficient. For example, when $\mathbf{m}_i^0$ lies in the $xy$ plane we can choose $\hat{n}_i = \hat{z}$. However, when considering domain wall or other interface configurations $\hat{n}_i$ should be chosen specifically. Using $\hat{n}_i$ one can define a site-dependent basis for $\delta\mathbf{m}_i$ in the plane orthogonal to $\mathbf{m}_i^0$:

$$\hat{n}_i^1 \equiv \frac{\hat{n}_i \times \mathbf{m}_i^0}{|\hat{n}_i \times \mathbf{m}_i^0|}\ ,\ \hat{n}_i^2 \equiv \mathbf{m}_i^0 \times \hat{n}_i^1 \tag{48}$$

such that

$$\delta\mathbf{m}_i = \delta m_i^1 \hat{n}_i^1 + \delta m_i^2 \hat{n}_i^2 \tag{49}$$

In this basis, the linearized LLG equation has the same dimension as the transverse degrees of freedom of the spins and can be written as

$$\sum_{j,b}[G^{-1}(\omega)]_{ia,jb}\delta m_j^b = -\gamma(\hat{n}_i^a \times \mathbf{m}_i^0)\cdot\mathbf{h}_i^{\text{ext}} \tag{50}$$

where

$$[G^{-1}(\omega)]_{ia,jb} = -i\omega\delta_{ij}(\delta_{ab} + \alpha\epsilon_{ab}) - \gamma\epsilon_{ab}\left(\mathbf{m}_i^0 \cdot \frac{\partial H}{\partial\mathbf{m}_i^0}\right) - \gamma(\hat{n}_i^a \times \mathbf{m}_i^0)\cdot\left(\frac{\partial^2 H}{\partial\mathbf{m}_i^0\partial\mathbf{m}_j^0}\cdot\hat{n}_j^b\right) \tag{51}$$

where $\epsilon_{ab}$ is the two-dimension Levi-Civita symbol. Then for a given $\mathbf{h}_i^{\text{ext}}$, $\delta\mathbf{m}_i(\omega)$ can be obtained by inverting Eq. (50).

To calculate the spin current and the driving force from $\delta\mathbf{m}_i(\omega)$, we first note that for the kagome models we have

$$\begin{aligned}\Gamma_{ab}^{\gamma\beta} &= -\frac{\sqrt{3}JS^2}{3}\left(e_1^a e_1^b n_1^\gamma n_2^\beta + e_3^a e_3^b n_1^\gamma n_3^\beta + e_1^a e_1^b n_2^\gamma n_1^\beta + e_2^a e_2^b n_2^\gamma n_3^\beta + e_3^a e_3^b n_3^\gamma n_1^\beta + e_2^a e_2^b n_3^\gamma n_2^\beta\right) \\ &= -\frac{\sqrt{3}JS^2}{3}\sum_{i=1}^{3} e_i^a e_i^b \left(n_i^\gamma n_{[i+1]_3}^\beta + n_i^\beta n_{[i+1]_3}^\gamma\right)\end{aligned} \tag{52}$$

where the $\hat{e}_i$ and $\hat{n}_i$ vectors are defined similar to that in [2]. Denoting $R\hat{n}_i$ as $\hat{m}_i$, we have

$$\begin{aligned}\mathcal{J}_a^\alpha &= \frac{\sqrt{3}JS^2}{6}\epsilon_{\alpha\delta\lambda}\sum_{i=1}^{3} e_i^a e_i^b\left(m_i^\delta \partial_b m_{[i+1]_3}^\lambda + m_{[i+1]_3}^\delta \partial_b m_i^\lambda\right) \\ &= \frac{\sqrt{3}JS^2}{6}\sum_{i=1}^{3} e_i^a \left[\hat{m}_i \times (\hat{e}_i\cdot\nabla)\hat{m}_{[i+1]_3} + \hat{m}_{[i+1]_3}\times(\hat{e}_i\cdot\nabla)\hat{m}_i\right]_\alpha\end{aligned} \tag{53}$$

When $\hat{m}_i(\mathbf{r},t)=\hat{n}_i+\boldsymbol{\delta}\mathbf{m}_i(\mathbf{r},t)$ so that $\boldsymbol{\delta}\mathbf{m}_i$ is infinitesimal and $\boldsymbol{\delta}\mathbf{m}_i(\mathbf{r},t)=\mathrm{Re}[\boldsymbol{\delta}\mathbf{m}_i(\mathbf{r})e^{-i\omega t}]$, with the complex $\boldsymbol{\delta}\mathbf{m}_i(\mathbf{r})$ solved from the linearized LLG equation, we have the dynamical d.c. spin current

$$\begin{aligned}\langle\mathcal{J}_a^\alpha\rangle &= \frac{\sqrt{3}JS^2}{6}\sum_{i=1}^{3}e_i^a\Big\langle\hat{m}_i\times(\hat{e}_i\cdot\nabla)\hat{m}_{[i+1]_3}+\hat{m}_{[i+1]_3}\times(\hat{e}_i\cdot\nabla)\hat{m}_i\Big\rangle_\alpha \\ &= \frac{\sqrt{3}JS^2}{12}\sum_{i=1}^{3}e_i^a\mathrm{Re}\left[\boldsymbol{\delta}\mathbf{m}_i\times(\hat{e}_i\cdot\nabla)\boldsymbol{\delta}\mathbf{m}^*_{[i+1]_3}+\boldsymbol{\delta}\mathbf{m}_{[i+1]_3}\times(\hat{e}_i\cdot\nabla)\boldsymbol{\delta}\mathbf{m}^*_i\right]_\alpha\end{aligned} \tag{54}$$

where $\nabla\boldsymbol{\delta}\mathbf{m}_i$ can be approximated by finite difference.

$P$ is defined as

$$P_b^\gamma=-\frac{1}{4}\mathrm{Re}(\boldsymbol{\theta}\times\partial_b\boldsymbol{\theta}^*)_\gamma \tag{55}$$

The key is therefore to express $\boldsymbol{\theta}$, supposedly defined for each kagome unit cell, in terms of $\boldsymbol{\delta}\mathbf{m}_i$. To this end we note

$$\boldsymbol{\delta}\mathbf{m}_i=(R-\mathbb{I})\hat{n}_i=\boldsymbol{\theta}\times\hat{n}_i \tag{56}$$

Therefore

$$\hat{n}_i\times\boldsymbol{\delta}\mathbf{m}_i=\boldsymbol{\theta}-\hat{n}_i(\hat{n}_i\cdot\boldsymbol{\theta}) \tag{57}$$

and

$$\theta_\alpha\sum_i(\delta_{\alpha\beta}-n_i^\alpha n_i^\beta)\equiv 3(T\cdot\boldsymbol{\theta})_\beta=\sum_i(\hat{n}_i\times\boldsymbol{\delta}\mathbf{m}_i)_\beta \tag{58}$$

where $T_{\alpha\beta}=\delta_{\alpha\beta}-\frac{1}{3}\sum_i n_i^\alpha n_i^\beta$ can be position dependent. Therefore

$$\boldsymbol{\theta}=\frac{1}{3}T^{-1}\cdot\sum_i(\hat{n}_i\times\boldsymbol{\delta}\mathbf{m}_i). \tag{59}$$

When applying Eq. (54) to numerical calculations, one should note that it was obtained from the low-energy Lagrangian of the kagome models and is therefore valid only for Goldstone modes due to spontaneous breaking of the continuous rotation symmetry. However, $\boldsymbol{\delta}\mathbf{m}_i$ solved from the linearized LLG equation applied to a finite discrete spin model generally includes contributions different from the Goldstone modes. In practice this means $\boldsymbol{\delta}\mathbf{m}_i\neq\boldsymbol{\theta}\times\hat{n}_i$ using the $\boldsymbol{\theta}$ defined in Eq. (59). Therefore instead of using $\boldsymbol{\delta}\mathbf{m}_i$ directly in Eq. (54) we should replace them by

$$\boldsymbol{\delta}\tilde{\mathbf{m}}_i\equiv\boldsymbol{\theta}\times\hat{n}_i \tag{60}$$

to effectively filter out the irrelevant contributions.

## V. INJECTION OF MAGNONS FROM FM TO NONCOLLINEAR AFM

In this section we discuss how spin waves in an FM can be injected into a neighboring noncollinear AFM using a 1D scattering approach. For simplicity we ignore any anisotropy in the bulk.

For an FM on a given lattice, doing coarse graining in a similar way as that for the AFM leads to the LLG equation of the order parameter $\mathbf{m}$

$$\dot{\mathbf{m}}=-\gamma\mathbf{m}\times J\nabla^2\mathbf{m} \tag{61}$$

To get the FM wave equation, we linearize Eq. (61) by assuming

$$\mathbf{m}=\mathbf{m}_0+\boldsymbol{\delta}\mathbf{m},\ \ |\mathbf{m}_0|=1,\ \ \boldsymbol{\delta}\mathbf{m}\cdot\mathbf{m}_0=0 \tag{62}$$

Namely

$$\mathbf{m}_0\equiv\hat{n}_3,\ \ \boldsymbol{\delta}\mathbf{m}=\delta m_1\hat{n}_1+\delta m_2\hat{n}_2 \tag{63}$$

where $\hat{n}_{1,2,3}$ form a right-handed triad of unit vectors. Then it is easy to get the spin wave dispersion $\omega_\pm(k) = \pm\gamma J k^2$ and the corresponding eigensolutions:

$$\begin{pmatrix}\delta m_1\\ \delta m_2\end{pmatrix}_+ = \delta m_+ \begin{pmatrix}1\\ i\end{pmatrix}, \quad \begin{pmatrix}\delta m_1\\ \delta m_2\end{pmatrix}_- = \delta m_- \begin{pmatrix}1\\ -i\end{pmatrix} \tag{64}$$

We next consider noncollinear AFM, for which we directly linearize its Lagrangian, assuming the paramagnetic susceptibility to be isotropic:

$$\mathcal{L} = \frac{\rho}{2}\dot{\theta}_\alpha\dot{\theta}_\alpha + \frac{1}{4}\left(\Gamma^{\alpha\beta}_{ab}\partial_a\theta_\beta\partial_b\theta_\alpha - \Gamma^{\alpha\alpha}_{ab}\partial_a\theta_\beta\partial_b\theta_\beta\right). \tag{65}$$

The Euler-Lagrange equation is

$$\rho\ddot{\theta}_\gamma + \frac{1}{2}\left(\Gamma^{\alpha\gamma}_{ab}\partial_a\partial_b\theta_\alpha - \Gamma^{\alpha\alpha}_{ab}\partial_a\partial_b\theta_\gamma\right) = 0 \tag{66}$$

If considering a 1D scattering problem so that $\theta_\alpha = \theta_\alpha e^{i(kx-\omega t)}$, we can rewrite Eq. (66) as

$$-\omega^2\rho\theta_\gamma - \frac{k^2}{2}\left(\Gamma^{\alpha\gamma}_{xx}\theta_\alpha - \Gamma^{\alpha\alpha}_{xx}\theta_\gamma\right) = 0 \tag{67}$$

For the two noncollinear kagome AFM models considered in this work, when the spatial indices are $xx$, the spin indices must be $xx$ as well, i.e.

$$\Gamma^{xx}_{xx} = \eta\frac{\sqrt{3}}{2}JS^2 = \frac{\sqrt{3}}{2}JS^2 \tag{68}$$

Eq. (67) then becomes diagonal and gives one flat band and two linearly dispersive bands for both AFM order:

$$\omega_1 = 0,\ \omega_{2,3} = \sqrt{\frac{\rho}{2}\Gamma^{xx}_{xx}}k \tag{69}$$

with the corresponding solutions for $\theta$:

$$\theta_1 = \theta\begin{pmatrix}1\\0\\0\end{pmatrix},\ \theta_2 = \theta\begin{pmatrix}0\\1\\0\end{pmatrix},\ \theta_3 = \theta\begin{pmatrix}0\\0\\1\end{pmatrix} \tag{70}$$

Now consider an FM/AFM interface located at $x = 0$. In the $x < 0$ region the solution is

$$\psi(x) = \psi^{\mathrm{F}}_+ + r\psi^{\mathrm{F}}_- \tag{71}$$

In the $x > 0$ region the solution is

$$\psi(x) = t_1\psi^{\mathrm{AF}}_1 + t_2\psi^{\mathrm{AF}}_2 + t_3\psi^{\mathrm{AF}}_3. \tag{72}$$

In the above equations, $r$ is the reflection coefficient, $t_{1,2,3}$ are the transmission coefficients, $\psi^{\mathrm{F}}_+$ is the + branch spin wave in the FM, propagating to the right, and properly normalized. For example

$$\psi^{\mathrm{F}}_+ \equiv \frac{1}{\sqrt{2}}\delta m\begin{pmatrix}1\\ i\end{pmatrix} e^{i[kx-\omega_+(k)t]} \tag{73}$$

where the basis of the column vector is the Cartesian components along $\hat{n}_{1,2}$ defined in Eq. (63). Consequently

$$\psi^{\mathrm{F}}_- \equiv \frac{1}{\sqrt{2}}\delta m\begin{pmatrix}1\\ -i\end{pmatrix} e^{i[kx-\omega_-(k)t]} = \frac{1}{\sqrt{2}}\delta m\begin{pmatrix}1\\ -i\end{pmatrix} e^{i[kx+\omega_+(k)t]} \tag{74}$$

Namely, $\psi^{\mathrm{F}}_-$ is a left-going spin wave of the same energy as the right-going $\psi^{\mathrm{F}}_+$. $\psi^{\mathrm{AF}}_{1,2,3}$ are similarly defined as

$$\psi^{\mathrm{AF}}_1 \equiv \theta\begin{pmatrix}1\\0\\0\end{pmatrix} e^{i[kx-\omega_1(k)t]},\ \psi^{\mathrm{AF}}_2 \equiv \theta\begin{pmatrix}0\\1\\0\end{pmatrix} e^{i[kx-\omega_2(k)t]},\ \psi^{\mathrm{AF}}_3 \equiv \theta\begin{pmatrix}0\\0\\1\end{pmatrix} e^{i[kx-\omega_3(k)t]} \tag{75}$$

To proceed, we need to find the boundary condition at the FM/AFM interface that relates $\psi(x=0^-)$ to $\psi(x=0^+)$. This is obtained from the linearized equations of motion of $\delta\mathbf{m}$ and $\boldsymbol{\theta}$ at the interface, which in turn must be obtained by coarse-graining the original Heisenberg models at the interface. Here we follow the idea of [10] and adopt a first approximation of the boundary condition by ignoring any gradient terms in the coarse-grained interface Lagrangian, which is reduced to a phenomenological interface energy term

$$U_{\mathrm{i}} = \delta(x) E_s (\mathbf{m}^{\mathrm{F}} \cdot \mathbf{m}^{\mathrm{AF}} + \mathbf{m}^{\mathrm{F}} \cdot R^{\mathrm{AF}} \cdot \boldsymbol{\alpha}) \tag{76}$$

where the constant $E_s$ is related to the strength of the interface exchange coupling, $\mathbf{m}^{\mathrm{F}}$ and $\mathbf{m}^{\mathrm{AF}}$ are the (net) magnetizations of the FM and the AFM, respectively, $R^{\mathrm{AF}}$ is the rotation matrix or the spin frame vectors for the AFM, and the vector $\boldsymbol{\alpha}$ depends on the interface details.

Adding the above $U_{\mathrm{i}}$ to the LLG equation for $\mathbf{m}^{\mathrm{F}}$, integrating the resulting LLG equation in a thin layer across the interface, retaining only the terms that become abnormally large due to discontinuities at the interface, and approximating $\mathbf{m}^{\mathrm{AF}} = \rho\boldsymbol{\Omega}$, we obtain the first set of boundary conditions

$$\left[ J\partial_x \mathbf{m}^{\mathrm{F}} + E_s \left( \rho\dot{\boldsymbol{\theta}} + \boldsymbol{\theta} \times \boldsymbol{\alpha} \right) \right] \Big|_{x=0} = 0 \tag{77}$$

or equivalently (neglecting the $|_{x=0}$ for brevity),

$$\begin{aligned} &\rho\dot{\theta}_x + \theta_y\alpha_z - \theta_z\alpha_y = 0 \\ &J\partial_x m_y^{\mathrm{F}} + E_s(\rho\dot{\theta}_y + \theta_z\alpha_x - \theta_x\alpha_z) = 0 \\ &J\partial_x m_z^{\mathrm{F}} + E_s(\rho\dot{\theta}_z + \theta_x\alpha_y - \theta_y\alpha_x) = 0 \end{aligned} \tag{78}$$

On the other hand, $U_{\mathrm{i}}$ also changes the equations of motion on the AF side. Following a similar procedure as above we obtain the second set of boundary conditions

$$\left( -\frac{1}{2}\Gamma^{xx}_{xx}\partial_x\theta_x\delta_{\alpha x} + \frac{1}{2}\Gamma^{xx}_{xx}\partial_x\theta_\alpha - E_s\epsilon_{\alpha\beta\gamma}\alpha_\beta\dot{m}^{\mathrm{F}}_\gamma + E_s\rho\dot{m}^{\mathrm{F}}_\alpha \right) \Big|_{x=0} = 0 \tag{79}$$

or equivalently

$$\begin{aligned} &\alpha_y\dot{m}^{\mathrm{F}}_z - \alpha_z\dot{m}^{\mathrm{F}}_y = 0 \\ &\frac{1}{2}\Gamma^{xx}_{xx}\partial_x\theta_y + E_s\alpha_x\dot{m}^{\mathrm{F}}_z + E_s\rho\dot{m}^{\mathrm{F}}_y = 0 \\ &\frac{1}{2}\Gamma^{xx}_{xx}\partial_x\theta_z - E_s\alpha_x\dot{m}^{\mathrm{F}}_y + E_s\rho\dot{m}^{\mathrm{F}}_z = 0 \end{aligned} \tag{80}$$

To get some feel of the physics behind the boundary condition Eqs. (78) and (80), let us consider the simpler case of $\boldsymbol{\alpha} = 0$, meaning the orientation of the noncollinear order does not couple to the magnetization of the ferromagnet linearly. Then the first equation in Eq. (80) becomes trivial, and the first equation in Eq. (78) requires $\dot{\theta}_x$ to vanish. Namely no spin waves for the flat band are excited. The 2nd and 3rd equations in Eq. (80) can be viewed as continuity equations–the time derivative of $m^{\mathrm{F}}_{y,z}$, related to that of the angular frequency, is converted to the spin current for $y, z$ spins on the AFM side. The 2nd and 3rd equations in Eq. (78) describe a related but different effect on the FM side: the canting field on the AFM side ($\rho\dot{\theta}$) is balanced by the effective magnetic field integrated over the interface layer on the FM side.

In the other limit, i.e. when $U_{\mathrm{i}}$ is dominated by the $\boldsymbol{\alpha}$ term, we have

$$\begin{aligned} &\alpha_y\dot{m}^{\mathrm{F}}_z - \alpha_z\dot{m}^{\mathrm{F}}_y = 0 \\ &\frac{1}{2}\Gamma^{xx}_{xx}\partial_x\theta_y + E_s\alpha_x\dot{m}^{\mathrm{F}}_z = 0 \\ &\frac{1}{2}\Gamma^{xx}_{xx}\partial_x\theta_z - E_s\alpha_x\dot{m}^{\mathrm{F}}_y = 0 \\ &\rho\dot{\theta}_x + \theta_y\alpha_z - \theta_z\alpha_y = 0 \\ &J\partial_x m_y^{\mathrm{F}} + E_s(\theta_z\alpha_x - \theta_x\alpha_z) = 0 \\ &J\partial_x m_z^{\mathrm{F}} + E_s(\theta_x\alpha_y - \theta_y\alpha_x) = 0 \end{aligned} \tag{81}$$

However, the first equation requires the reflection coefficient $r = \pm 1$ and either $\alpha_y$ or $\alpha_z$ must vanish, because $\boldsymbol{\alpha}$ is real. Moreover, since $\dot{\theta}_x = 0$ for general $\omega \neq 0$, the 4th equation means that the transmitted spin waves must be

linearly polarized. Therefore the presence of $\boldsymbol{\alpha}$ is highly undesirable. In practice this means that one should try to have a fully compensated interface of the AFM so that the orientation of the noncollinear order parameter is not coupled linearly to $\mathbf{m}^{\mathrm{F}}$. This is the main criterion we used when designing our interface for the numerical calculations of the FM/AFM interface.

## VI. DERIVATION OF THE GENERAL FORMULA OF $\Gamma$

In this section we derive the general formula of $\Gamma$ and discuss its symmetry properties. Consider a general Heisenberg spin Hamiltonian defined on certain lattice

$$H = \frac{1}{2}\sum_{ij,pq} J_{ip,jq}\mathbf{S}_{ip}\cdot\mathbf{S}_{jq} \tag{82}$$

where $i, j$ label the lattice unit cell and $p, q$ label sublattices within each unit cell. An arbitrary state of the system can be obtained by a position-dependent rotation matrix acting on the ground state spins $\mathbf{S}^0_{ip} = S\hat{\mathbf{m}}_p$, where $\hat{\mathbf{m}}_p$ are unit vectors. Namely,

$$\mathbf{S}_{ip} = SR(\mathbf{r}_{ip})\hat{\mathbf{m}}_p \tag{83}$$

For slow spatial variation of $R$, we can perform gradient expansion as

$$R(\mathbf{r}_{ip}+\delta\mathbf{r}) = R(\mathbf{r}_{ip}) + (\delta\mathbf{r}\cdot\nabla)R(\mathbf{r}_{ip}) + \frac{1}{2}(\delta\mathbf{r}\cdot\nabla)^2R(\mathbf{r}_{ip}) + \ldots \tag{84}$$

Applying the above expansion to Eq. (82) and keeping up to second order in spatial gradient terms only, we get

$$\begin{aligned} H \;\approx\; & \frac{S^2}{2}\sum_{ip,jq} J_{ip,jq}\hat{\mathbf{m}}_p\cdot\hat{\mathbf{m}}_q \\ &+ \frac{S^2}{2}\sum_{ip,jq} J_{ip,jq}R\hat{\mathbf{m}}_p\cdot(\mathbf{r}_{ip,jq}\cdot\nabla)R\hat{\mathbf{m}}_q \\ &+ \frac{S^2}{4}\sum_{ip,jq} J_{ip,jq}R\hat{\mathbf{m}}_p\cdot(\mathbf{r}_{ip,jq}\cdot\nabla)^2R\hat{\mathbf{m}}_q \end{aligned} \tag{85}$$

where $\mathbf{r}_{ip,jq} \equiv \mathbf{r}_{jq} - \mathbf{r}_{ip}$ is the vector pointing from site $ip$ to site $jq$, and $R = R(\mathbf{r}_{ip})$. We then look at each term individually. Start with the first order term:

$$\begin{aligned} \frac{S^2}{2}\sum_{ip,jq} J_{ip,jq}(R\hat{\mathbf{m}}_p)\cdot[(\mathbf{r}_{ip,jq})_a(\partial_aR)\hat{\mathbf{m}}_q] &= \frac{S^2}{2}\sum_{ip,jq} J_{ip,jq}R_{bc}(\hat{\mathbf{m}}_p)_c(\mathbf{r}_{ip,jq})_a(\partial_aR)_{bd}(\hat{\mathbf{m}}_q)_d \\ &= \frac{S^2}{2}\sum_{ip,jq} J_{ip,jq}(R^{-1}\partial_aR)_{cd}(\mathbf{r}_{ip,jq})_a(\hat{\mathbf{m}}_p)_c(\hat{\mathbf{m}}_q)_d \end{aligned} \tag{86}$$

To coarse-grain such a term, we assume $R(\mathbf{r}_{ip})$ to be independent of the sublattice index $p$. This is equivalent to assuming that the rotation varies with a length scale much larger than the unit cell size. We can thus replace the sum over unit cells $i$ by integration with a factor of the unit cell volume $V_c$

$$\frac{S^2}{2}\sum_{ip,jq} J_{ip,jq}(R\hat{\mathbf{m}}_p)\cdot[(\mathbf{r}_{ip,jq})_a(\partial_aR)\hat{\mathbf{m}}_q] \;\approx\; \frac{S^2}{2V_c}\int d^3\mathbf{r}(R^{-1}\partial_aR)_{cd}\sum_{p,jq} J_{0p,jq}(\mathbf{r}_{0p,jq})_a(\hat{\mathbf{m}}_p)_c(\hat{\mathbf{m}}_q)_d \tag{87}$$

where $J_{0p,jq}$ is the exchange coupling between sublattice $p$ in the the unit cell at the origin and sublattice $q$ in unit cell $j$. In other words $J_{0p,jq} = J_{pq}(0,\mathbf{R}_j)$, with $\mathbf{R}_j$ a Bravais lattice vector. Furthermore, $J$ must obey translation symmetry, so

$$J_{pq}(0,\mathbf{R}_j) = J_{qp}(0,-\mathbf{R}_j) = J_{qp}(0,\mathbf{R}_{j'}) \tag{88}$$

and since

$$\mathbf{r}_{0p,jq} = \boldsymbol{\tau}_q + \mathbf{R}_j - \boldsymbol{\tau}_p = -\mathbf{r}_{0q,j'p} \tag{89}$$

we obtain

$$\sum_{p,jq} J_{0p,jq}(\mathbf{r}_{0p,jq})_a(\hat{\mathbf{m}}_p)_c(\hat{\mathbf{m}}_q)_d = -\sum_{p,j'q} J_{0q,j'p}(\mathbf{r}_{0q,j'p})_a(\hat{\mathbf{m}}_q)_c(\hat{\mathbf{m}}_p)_d \tag{90}$$

If this sum is defined as $A_{acd}$, the above equation means $A_{acd} = -A_{adc}$, i.e., the diagonal part of $A_a$ always vanishes. Furthermore, if the magnetic order has spatial inversion symmetry, one can show that $A_{acd} = -A_{acd} = 0$. Thus we do not need to consider the first order term in systems with inversion symmetry.

The second order term is:

$$\frac{S^2}{4}\sum_{ip,jq} J_{ip,jq}(R\hat{\mathbf{m}}_p)\cdot\left[(\mathbf{r}_{ip,jq}\cdot\nabla)^2 R\hat{\mathbf{m}}_q\right] \approx \frac{S^2}{4V_c}\int d^3\mathbf{r}\,\left(R^{-1}\partial_a\partial_b R\right)_{\alpha\beta}\sum_{p,jq} J_{0p,jq}(\mathbf{r}_{0p,jq})_a(\mathbf{r}_{0p,jq})_b(\hat{\mathbf{m}}_p)_\alpha(\hat{\mathbf{m}}_q)_\beta \tag{91}$$

We can therefore define $\Gamma$ as

$$\Gamma_{ab}^{\alpha\beta} = -\frac{S^2}{V_c}\sum_{p,jq} J_{0p,jq}(\mathbf{r}_{0p,jq})_a(\mathbf{r}_{0p,jq})_b(\hat{\mathbf{m}}_p)_\alpha(\hat{\mathbf{m}}_q)_\beta \tag{92}$$

which is symmetric under $a \leftrightarrow b$ and $\alpha \leftrightarrow \beta$. The former is trivial and the latter can be proven similar to the steps leading to Eq. (90). Using this property, together with the fact that $\partial_a(R^{-1}\partial_b R)_{\alpha\beta} = -\partial_a(R^{-1}\partial_b R)_{\beta\alpha}$, we can finally rewrite the second order term as

$$-\frac{1}{4}\int d^3\mathbf{r}\Gamma_{ab}^{\alpha\beta}\left[(R^{-1}\partial_a R)(R^{-1}\partial_b R)\right]_{\alpha\beta} \tag{93}$$

Eq. (92) is independent of unit cell choices as long as the number of sublattices does not change. Choosing different unit cells amounts to shifting positions of certain sublattices by nonzero Bravais lattice vectors, or relabels $ip$ as $i'p'$. However, since each term in Eq. (92) only depends on the relative positions of two sublattices, it is independent of unit cell choices. Therefore $\Gamma$ is also independent of unit cell choices.

Since Eq. (93) must be a scalar, $\Gamma$ is a rank-4 Cartesian tensor, which means it transforms under $O(3)$ operation $O$ as

$$(\Gamma')_{ij}^{\eta\nu} = O_{ia}O_{jb}O_{\eta\alpha}O_{\nu\beta}\Gamma_{ab}^{\alpha\beta} \tag{94}$$

where $\Gamma'$ means the $\Gamma$ tensor in the transformed coordinate system. Eq. (94) can then be used to find the symmetry constraints on $\Gamma$ if $O$ is a space group symmetry operation for a given system, under which $\Gamma' = \Gamma$.

The $\Gamma$ tensors for magnetic structures of $Mn_3Ir$ and $Mn_3Sn$ by considering nearest-neighbor exchange coupling and approximating the in-plane and out-of-plane nearest neighbor distances in $Mn_3Sn$ to be the same are listed below:

For $Mn_3Ir$:

$$\Gamma_{xx} = \frac{2Ja_0^2S^2}{3V_c}\begin{pmatrix} 4 & -2 & -2 \\ -2 & 1 & 1 \\ -2 & 1 & 1 \end{pmatrix} \tag{95}$$

$$\Gamma_{yy} = \frac{2Ja_0^2S^2}{3V_c}\begin{pmatrix} 1 & -2 & 1 \\ -2 & 4 & -2 \\ 1 & -2 & 1 \end{pmatrix} \tag{96}$$

$$\Gamma_{zz} = \frac{2Ja_0^2S^2}{3V_c}\begin{pmatrix} 1 & 1 & -2 \\ 1 & 1 & -2 \\ -2 & -2 & 4 \end{pmatrix} \tag{97}$$

For $Mn_3Sn$:

$$\Gamma_{xx} = \frac{2Ja_0^2S^2}{V_c}\begin{pmatrix}3&0&0\\0&1&0\\0&0&0\end{pmatrix} \tag{98}$$

$$\Gamma_{yy} = \frac{2Ja_0^2S^2}{V_c}\begin{pmatrix}1&0&0\\0&3&0\\0&0&0\end{pmatrix} \tag{99}$$

$$\Gamma_{zz} = \frac{4Ja_0^2S^2}{V_c}\begin{pmatrix}1&0&0\\0&1&0\\0&0&0\end{pmatrix} \tag{100}$$

$$\Gamma_{xy} = \Gamma_{yx} = \frac{2Ja_0^2S^2}{V_c}\begin{pmatrix}0&-1&0\\-1&0&0\\0&0&0\end{pmatrix} \tag{101}$$

$$\tag{102}$$

## VII. SPIN WAVES AND D.C. SPIN CURRENTS OF ISOTROPIC NONCOLLINEAR ANTIFERROMAGNETS

In this section we discuss spin waves of a general isotropic Heisenberg noncollinear antiferromagnet.

The angular average of $\Gamma$ is defined as:

$$\bar{\Gamma}^{\alpha\beta}_{ab} \equiv \frac{1}{8\pi^2}\int d\psi \int \sin\theta d\theta \int d\varphi\, (RRRR\Gamma)^{\alpha\beta}_{ab} \tag{103}$$

where $RRRR\Gamma$ means contracting the right index of each rotation matrix $R$ with a unique index of $\Gamma$. The result, given in the main text, can be obtained following the method in [11] and references therein.

We mention in passing that in the 2D case we found that

$$\bar{\Gamma}^{xy}_{xy} = \bar{\Gamma}^{xy}_{yx} = \bar{\Gamma}^{yx}_{xy} = \bar{\Gamma}^{yx}_{yx} = \frac{1}{4}\Gamma^{ab}_{ab} - \frac{1}{8}\Gamma^{aa}_{bb} \equiv g_{\rm H} \tag{104}$$

where $a, b$ run through $x, y$ and the angular averaging is with respect to rotation about $z$. However, in 2D components such as $\bar{\Gamma}^{xx}_{xy}$ are also nonzero since $\epsilon_{\alpha a}\delta_{\beta b}$ is isotropic. Such components may be identified as certain Hall effects as well, but we do not consider them in this work since they vanish for the kagome models studied here. Using Eq. (104) we can find that $g_{\rm H} = \frac{\sqrt{3}}{4}JS^2$ (0) for direct (inverse) triangular order on the kagome lattice. Although $g_{\rm H}$ may be different (such as for the inverse triangular order) from $\Gamma^{xy}_{xy}$ that gives the transverse spin currents in Fig. 2 of the main text, it is the part that is invariant as one rotates the kagome lattices together with the spin order.

To get the spin waves, we consider infinitesimal rotations $R_{\alpha\beta} = \delta_{\alpha\beta} - \theta_\gamma\epsilon_{\gamma\alpha\beta}$. Then the kinetic term in the Lagrangian becomes

$$\frac{\bar{\rho}}{4}{\rm Tr}(\partial_t R\partial_t R^{-1}) = \frac{\bar{\rho}}{2}\dot{\theta}_\alpha\dot{\theta}_\alpha \tag{105}$$

The potential energy term becomes

$$\begin{aligned}\frac{1}{4}\bar{\Gamma}^{\alpha\beta}_{ab}[(R^{-1}\partial_a R)(R^{-1}\partial_b R)]_{\alpha\beta} &= \frac{1}{4}\left(\bar{\Gamma}^{\alpha\beta}_{ab}\partial_a\theta_\beta\partial_b\theta_\alpha - \bar{\Gamma}^{\alpha\alpha}_{ab}\partial_a\theta_\beta\partial_b\theta_\beta\right) \\ &= \frac{1}{4}\left[g_{\rm H}(\partial_a\theta_b\partial_b\theta_a + \partial_a\theta_a\partial_b\theta_b) - 2(g_{\rm H}+g_0)\partial_a\theta_b\partial_a\theta_b\right]\end{aligned} \tag{106}$$

We next derive the equations of motion for the Lagrangian density in 3D

$$\mathcal{L} = \frac{\bar{\rho}}{2}\dot{\theta}_\alpha\dot{\theta}_\alpha + \frac{1}{4}\left[g_{\rm H}(\partial_a\theta_b\partial_b\theta_a + \partial_a\theta_a\partial_b\theta_b - 2\partial_a\theta_b\partial_a\theta_b) - 2g_0\partial_a\theta_b\partial_a\theta_b\right] \tag{107}$$

which have the form of the continuity equation

$$\partial_t(\bar{\rho}\partial_t\theta_\alpha) + \partial_i\left[\frac{1}{4}g_{\rm H}(2\partial_\alpha\theta_i + 2\partial_b\theta_b\delta_{\alpha i} - 4\partial_i\theta_\alpha) - g_0\partial_i\theta_\alpha\right] = 0 \tag{108}$$

or equivalently

$$\bar{\rho}\partial_t^2\theta_\alpha + g_{\rm H}(\partial_\alpha\nabla\cdot\boldsymbol{\theta} - \nabla^2\theta_\alpha) - g_0\nabla^2\theta_\alpha = 0 \tag{109}$$

Consider plane wave solutions $\boldsymbol{\theta}(\mathbf{r},t) = \boldsymbol{\theta}e^{i(\mathbf{k}\cdot\mathbf{r}-\omega t)}$, the above equations of motion lead to

$$\left[-\bar{\rho}\omega^2 + (g_{\rm H}+g_0)k^2\right]\theta_\alpha - g_{\rm H}k_\alpha k_\beta\theta_\beta = 0 \tag{110}$$

The corresponding secular equation is found to be

$$[\bar{\rho}\omega^2 - (g_{\rm H}+g_0)k^2]^2(\bar{\rho}\omega^2 - g_0k^2) = 0 \tag{111}$$

which has the solutions

$$\begin{aligned} \omega &= c_{\rm I,II,III}k, \\ c_{\rm I} &= \sqrt{\frac{g_0}{\bar{\rho}}}, \\ c_{\rm II} = c_{\rm III} &= \sqrt{\frac{g_{\rm H}+g_0}{\bar{\rho}}}. \end{aligned} \tag{112}$$

The three modes are respectively a longitudinal and two transverse modes, which can be explicitly seen from their eigenvectors. Therefore for general isotropic noncollinear AFM in 3D, two transverse spin wave branches are always degenerate, similar to phonons in isotropic elastic media.

We next consider the d.c. spin current due to spin waves in the 3D isotropic case. Without loss of generality we assume the spin wave to be propagating along $x$ and is a linear superposition of the two transverse modes, i.e.,

$$\boldsymbol{\theta}(x,t) = \mathrm{Re}\left[(\theta_y\hat{y} + \theta_z\hat{z})e^{ik(x-ct)}\right] \tag{113}$$

where $c = \sqrt{(g_0+g_{\rm H})/\bar{\rho}}$ and $\theta_{y,z}$ are complex numbers. We then have

$$\langle(R^{-1}L^\alpha\partial_bR)_{\beta\gamma}\rangle_t = -\delta_{bx}\delta_{\alpha\gamma}\delta_{\beta x}k\mathrm{Im}(\theta_y\theta_z^*) \tag{114}$$

where we have omitted a term that is antisymmetric under $\beta\leftrightarrow\gamma$ due to the symmetry of $\Gamma$. As a result, the time-averaged spin current becomes

$$\mathcal{J}_a^\alpha = \frac{1}{2}\bar{\Gamma}_{ab}^{\beta\gamma}\langle(R^{-1}L^\alpha\partial_bR)_{\beta\gamma}\rangle_t = -\frac{1}{2}\bar{\Gamma}_{ax}^{\alpha x}k\mathrm{Im}(\theta_y\theta_z^*) \tag{115}$$

which also means that the driving force $P_x^x = -\frac{1}{2}k\mathrm{Im}(\theta_y\theta_z^*)$. Using the isotropic $\bar{\Gamma}$, we have

$$\mathcal{J}_a^\alpha = -\frac{1}{2}\left[g_{\rm H}(\delta_{\alpha a} + \delta_{ax}\delta_{\alpha x}) + g_0\delta_{ax}\delta_{\alpha x}\right]k\mathrm{Im}(\theta_y\theta_z^*) \tag{116}$$

Therefore

$$\begin{aligned} \mathcal{J}_x^x &= -\frac{g_0+2g_{\rm H}}{2}k\mathrm{Im}(\theta_y\theta_z^*), \\ \mathcal{J}_y^y = \mathcal{J}_z^z &= -\frac{g_{\rm H}}{2}k\mathrm{Im}(\theta_y\theta_z^*) \end{aligned} \tag{117}$$

with all the other components vanishing.


[1] T. Dombre and N. Read, Nonlinear $\sigma$ models for triangular quantum antiferromagnets, Phys. Rev. B **39**, 6797 (1989).
[2] C. Ulloa and A. S. Nunez, Solitonlike magnetization textures in noncollinear antiferromagnets, Phys. Rev. B **93**, 134429 (2016).
[3] B. Li and A. A. Kovalev, Spin superfluidity in noncollinear antiferromagnets, Phys. Rev. B **103**, L060406 (2021).
[4] M. A. Lund, A. Salimath, and K. M. D. Hals, Spin pumping in noncollinear antiferromagnets, Phys. Rev. B **104**, 174424 (2021).

[5] D. R. Rodrigues, A. Salimath, K. Everschor-Sitte, and K. M. D. Hals, Dzyaloshinskii-Moriya induced spin-transfer torques in kagome antiferromagnets, Phys. Rev. B **105**, 174401 (2022).
[6] B. Pradenas and O. Tchernyshyov, Spin-frame field theory of a three-sublattice antiferromagnet, Phys. Rev. Lett. **132**, 096703 (2024).
[7] A. Altland and B. D. Simons, *Condensed Matter Field Theory*, 3rd ed. (Cambridge University Press, 2023).
[8] N. Marzari and D. Vanderbilt, Maximally localized generalized Wannier functions for composite energy bands, Phys. Rev. B **56**, 12847 (1997).
[9] D. Hill, V. Slastikov, and O. Tchernyshyov, Chiral magnetism: a geometric perspective, SciPost Phys. **10**, 078 (2021).
[10] R. Khymyn, I. Lisenkov, V. S. Tiberkevich, A. N. Slavin, and B. A. Ivanov, Transformation of spin current by antiferromagnetic insulators, Phys. Rev. B **93**, 224421 (2016).
[11] E. A. Power and T. Thirunamachandran, Circular dichroism: A general theory based on quantum electrodynamics, The Journal of Chemical Physics **60**, 3695 (2003), https://pubs.aip.org/aip/jcp/article-pdf/60/9/3695/11153635/3695_1_online.pdf.
